# Supplementary material for: Exact conditional calibration of residual processes in linear mixed models
Source: arXiv:2611.40832 source file (2026-11-30)
Supplement: Supplementary file 1 [file labels-supplement.tex]

\makeatletter
\global\@namedef{r@S-tab:guide}{{S1}{1}{Where each numbered statement of the paper is proved, and the related statements of this supplement}{table.1}{supplement.pdf}}
\global\@namedef{r@S-sec:si-exact}{{S1}{2}{Proofs of the exact results}{section.1}{supplement.pdf}}
\global\@namedef{r@S-prop:exact-F}{{S1}{2}{The primary fixed-part process}{theorem.1}{supplement.pdf}}
\global\@namedef{r@S-tab:gaussian-failure}{{S2}{3}{Two constructed null cases in which unrescaled Gaussian draws (G) for $O$ fail and the exact test (E) does not: sizes at $\alpha =0.05$ over 2000 replicates (ML fits, $B=999$, indicator weights I and the minimum-$p$ rule D), with the mean and the 5\% and 95\% quantiles of the radial factor $d=\|\bm R\bm y\|/(\widehat \sigma \sqrt r)$ and the share of singular fits (sing.). Many fixed effects: $n=100$ in 20 subjects of 5 with a random intercept and $p=20$ (an intercept and 19 standard normal covariates); small residual dimension: $n=150$ in 50 subjects of 3 with random intercept and slope, $p=2$, $r=50$. Monte Carlo standard error 0.005 at 0.05}{table.2}{supplement.pdf}}
\global\@namedef{r@S-sec:setting}{{S2}{4}{Setting and conditions for the power results}{section.2}{supplement.pdf}}
\global\@namedef{r@S-sec:si-conditions}{{S2}{4}{Setting and conditions for the power results}{section.2}{supplement.pdf}}
\global\@namedef{r@S-sec:model}{{S2.1}{4}{Model, orderings and Gaussian draws}{subsection.2.1}{supplement.pdf}}
\global\@namedef{r@S-sec:processes}{{S2.1}{4}{Model, orderings and Gaussian draws}{subsection.2.1}{supplement.pdf}}
\global\@namedef{r@S-sec:tests}{{S2.1}{4}{Model, orderings and Gaussian draws}{subsection.2.1}{supplement.pdf}}
\global\@namedef{r@S-eq:P-annihilates}{{S1}{4}{Model, orderings and Gaussian draws}{equation.2.1}{supplement.pdf}}
\global\@namedef{r@S-eq:secondary-process}{{S2}{4}{Model, orderings and Gaussian draws}{equation.2.2}{supplement.pdf}}
\global\@namedef{r@S-eq:test-statistics}{{S3}{4}{Model, orderings and Gaussian draws}{equation.2.3}{supplement.pdf}}
\global\@namedef{r@S-sec:secondary}{{S2.2}{4}{Conditions on the secondary processes from Gaussian draws}{subsection.2.2}{supplement.pdf}}
\global\@namedef{r@S-eq:fitted-quantities}{{S4}{4}{Conditions on the secondary processes from Gaussian draws}{equation.2.4}{supplement.pdf}}
\global\@namedef{r@S-eq:secondary-identity}{{S5}{5}{Conditions on the secondary processes from Gaussian draws}{equation.2.5}{supplement.pdf}}
\global\@namedef{r@S-eq:universal-modulus-secondary}{{S6}{5}{Conditions on the secondary processes from Gaussian draws}{equation.2.6}{supplement.pdf}}
\global\@namedef{r@S-eq:secondary-linearity}{{S7}{5}{Conditions on the secondary processes from Gaussian draws}{equation.2.7}{supplement.pdf}}
\global\@namedef{r@S-sec:alternative-conditions}{{S2.3}{5}{Conditions under alternatives}{subsection.2.3}{supplement.pdf}}
\global\@namedef{r@S-eq:alternative-model}{{S8}{5}{Conditions under alternatives}{equation.2.8}{supplement.pdf}}
\global\@namedef{r@S-eq:mean-function}{{S9}{5}{Conditions under alternatives}{equation.2.9}{supplement.pdf}}
\global\@namedef{r@S-sec:si-grid}{{S3}{6}{Statistics on the fitted-value grid}{section.3}{supplement.pdf}}
\global\@namedef{r@S-sec:implemented-statistics}{{S3}{6}{Statistics on the fitted-value grid}{section.3}{supplement.pdf}}
\global\@namedef{r@S-eq:implemented-statistics}{{S10}{6}{Statistics on the fitted-value grid}{equation.3.10}{supplement.pdf}}
\global\@namedef{r@S-lem:implemented-indicator}{{S2}{6}{Exact indicator statistics with ties}{theorem.2}{supplement.pdf}}
\global\@namedef{r@S-sec:si-detection}{{S4}{7}{Behaviour under alternatives}{section.4}{supplement.pdf}}
\global\@namedef{r@S-sec:alternatives}{{S4}{7}{Behaviour under alternatives}{section.4}{supplement.pdf}}
\global\@namedef{r@S-sec:exact-power}{{S4.1}{7}{A finite-sample power bound for the exact tests}{subsection.4.1}{supplement.pdf}}
\global\@namedef{r@S-lem:exact-secondary-moment}{{S3}{7}{Mean square of the secondary statistics under rotations}{theorem.3}{supplement.pdf}}
\global\@namedef{r@S-thm:exact-power}{{S4}{8}{Power bound for the exact tests}{theorem.4}{supplement.pdf}}
\global\@namedef{r@S-thm:power}{{S5}{9}{Consistency for Gaussian draws}{theorem.5}{supplement.pdf}}
\global\@namedef{r@S-sec:exact-power-extension}{{S4.3}{10}{Root-CvM statistics and consistency of the exact tests}{subsection.4.3}{supplement.pdf}}
\global\@namedef{r@S-cor:exact-consistency}{{S6}{10}{Consistency of the exact tests}{theorem.6}{supplement.pdf}}
\global\@namedef{r@S-prop:mean-function}{{S7}{12}{Mean functions under Gaussian alternatives}{theorem.7}{supplement.pdf}}
\global\@namedef{r@S-eq:mean-function-formula}{{S11}{12}{Mean functions under Gaussian alternatives}{equation.4.11}{supplement.pdf}}
\global\@namedef{r@S-app:lemmas}{{S5}{13}{Auxiliary lemmas}{section.5}{supplement.pdf}}
\global\@namedef{r@S-lem:covering}{{S8}{13}{Quantile covering bound}{theorem.8}{supplement.pdf}}
\global\@namedef{r@S-lem:dyadic-modulus}{{S9}{13}{A finite-pattern Gaussian modulus}{theorem.9}{supplement.pdf}}
\global\@namedef{r@S-eq:dyadic-modulus}{{S12}{13}{A finite-pattern Gaussian modulus}{equation.5.12}{supplement.pdf}}
\global\@namedef{r@S-lem:anchored-supremum}{{S10}{14}{Supremum of an anchored sub-Gaussian process}{theorem.10}{supplement.pdf}}
\global\@namedef{r@S-sec:si-simulations}{{S6}{14}{Details of the simulation study}{section.6}{supplement.pdf}}
\global\@namedef{r@S-tab:designs}{{S3}{14}{The five designs and their fitted random structures under the null; $\bm R\bm y=\bm P\bm y$ when both covariates have a random slope at some level}{table.3}{supplement.pdf}}
\global\@namedef{r@S-fig:processes-example}{{S1}{15}{Processes of two simulated data sets from the nested design (subjects within centres, $n=16\,000$, one simulated data set drawn by the simulation code), with indicator weights, ML fits and $B=999$: (a) a quadratic mean term present in the data is omitted from the fit; (b) the centre slope is omitted from the fit. Black lines are the observed processes and grey bands the pointwise 2.5\% and 97.5\% quantiles of the secondary processes, Gaussian draws for $F$ and rotations for the projected processes, whose radial factors lie between 0.97 and 1.02 here. CvM $p$-values: (a) $F$ 0.001, $O$ 0.014, $O_1$ 0.002, $O_2$ 0.103; (b) $F$ 0.712, $O$ 0.001, $O_1$ 0.014, $O_2$ 0.003. A path leaving the band is not itself a rejection}{figure.1}{supplement.pdf}}
\global\@namedef{r@S-sec:si-rotation-check}{{S6.3}{16}{Rotation and numerical refitting}{subsection.6.3}{supplement.pdf}}
\global\@namedef{r@S-tab:rotation-refit}{{S4}{16}{Numerical rotation/refit check. Singular counts refer to the 50 original fits in each row. The last four columns are maximum relative changes over 150 rotations, with the scaling defined in the text}{table.4}{supplement.pdf}}
\global\@namedef{r@S-sec:si-exact-sim}{{S6.4}{16}{The exact tests}{subsection.6.4}{supplement.pdf}}
\global\@namedef{r@S-tab:projection-compare}{{S5}{17}{The exact test of the projected processes with the marks $\bm P\bm y$ of the one-level construction (P: $\bm P=\bm I-\bm Z\bm Z^+$, the offset $\bm c_O=\widehat \sigma ^{-1}\bm P\bm M\bm \Pi \bm y$ of Theorem~\ref {M-thm:exact-main} added to the observed and to every secondary mark vector) and with the marks $\bm R\bm y$ of the paper (R): CvM rejection rates at $\alpha =0.05$ and $n=4000$ on the first 1000 replicates and draws of the main study of the companion paper (ML fits, $B=999$), with indicator weights and the minimum-$p$ rule. The two coincide, $\bm R\bm y=\bm P\bm y$, in the nested, crossed and three-level designs under $H_0$ and under the omitted $x_1^2$, where both random slopes are fitted, and differ otherwise. Hypotheses and processes as in the main study of the companion paper; Monte Carlo standard error at most 0.016; leading zeros are omitted in the cells}{table.5}{supplement.pdf}}
\global\@namedef{r@S-tab:exact-single}{{S6}{18}{The exact tests in the single-level design: rejection rates at $\alpha =0.05$ of every process with indicator weights (I), the window $c=1$ and the minimum-$p$ rule (M), CvM and KS, 1000 replicates per cell}{table.6}{supplement.pdf}}
\global\@namedef{r@S-tab:exact-nested}{{S7}{18}{The exact tests in the nested design: rejection rates at $\alpha =0.05$ of every process with indicator weights (I), the window $c=1$ and the minimum-$p$ rule (M), CvM and KS, 1000 replicates per cell}{table.7}{supplement.pdf}}
\global\@namedef{r@S-tab:exact-crossed}{{S8}{19}{The exact tests in the crossed design: rejection rates at $\alpha =0.05$ of every process with indicator weights (I), the window $c=1$ and the minimum-$p$ rule (M), CvM and KS, 1000 replicates per cell}{table.8}{supplement.pdf}}
\global\@namedef{r@S-tab:exact-finite}{{S9}{19}{The exact tests in the five-centre design: rejection rates at $\alpha =0.05$ of every process with indicator weights (I), the window $c=1$ and the minimum-$p$ rule (M), CvM and KS, 1000 replicates per cell}{table.9}{supplement.pdf}}
\global\@namedef{r@S-tab:exact-three}{{S10}{19}{The exact tests in the three-level design: rejection rates at $\alpha =0.05$ of every process with indicator weights (I), the window $c=1$ and the minimum-$p$ rule (M), CvM and KS, 1000 replicates per cell}{table.10}{supplement.pdf}}
\global\@namedef{r@S-fig:overview}{{S2}{20}{CvM rejection rates of the exact tests against $n$ for every design (rows) and alternative (columns), indicator weights (dashed) and the minimum-$p$ rule (solid); 1000 replicates per point}{figure.2}{supplement.pdf}}
\global\@namedef{r@S-sec:si-small-r}{{S6.5}{21}{Calibrations along the residual dimension}{subsection.6.5}{supplement.pdf}}
\global\@namedef{r@S-tab:small-r-null}{{S11}{22}{Null rejection rates at $\alpha =0.05$ along the residual dimension $r$ (Section~\ref {sec:si-small-r}; CvM with the minimum-$p$ rule, $B=999$, 10\,000 replicates per row). E: rotations; $G_{\rm r}$: Gaussian draws with the marks divided by the residual standard deviation $\|\bm R\bm y\|/\sqrt r$; $G_{\widehat \sigma }$: Gaussian draws with the marks divided by $\widehat \sigma $ of the ML or of the REML fit. Situations: short series with a random slope, twenty fixed effects ($p=20$) and fixed effects in proportion ($p=n/5$). E and $G_{\rm r}$ are those of the ML fit. $\bar d$ is the mean radial factor and sing.\ the share of singular fits, both for ML. The Monte Carlo standard error is 0.002 at 0.05 and at most 0.005}{table.11}{supplement.pdf}}
\global\@namedef{r@S-tab:small-r-power}{{S12}{23}{Rejection rates at $\alpha =0.05$ under the omitted quadratic term along the residual dimension $r$ (Section~\ref {sec:si-small-r}; CvM with the minimum-$p$ rule, ML fits, $B=999$, 10\,000 replicates per row). E: rotations; $G_{\rm r}$: Gaussian draws with the marks divided by the residual standard deviation; E$-G_{\rm r}$ is their difference on the same replicates, with its paired standard error}{table.12}{supplement.pdf}}
\global\@namedef{r@S-tab:joint}{{S13}{23}{Family-wise rejection of the exact tests (CvM, $\alpha =0.05$, 1000 replicates per cell): the share of replicates in which some factor-specific test rejects (some $O_l$) and in which some test among $F_E$, $O_E$ and the $O_l$ rejects (any), with indicator weights (I) and the minimum-$p$ rule (D), and the rejection rates of the joint minimum-$p$ tests over the projected processes ($O$-joint) and over all processes including $F_E$ (all-joint), formed from the processes' indicator-weight columns (I) or from the processes and the five finite scales jointly (D) and calibrated by the same draws (Theorem~\ref {M-thm:exact-main} of the paper). Under $H_0$ the entries are sizes, under the alternatives powers; the single-level design has $O_1=O$}{table.13}{supplement.pdf}}
\global\@namedef{r@S-tab:power-n1000-4000}{{S14}{25}{Power of the exact tests at $n=1000$ and $4000$ (CvM, $\alpha =0.05$, 1000 replicates): $F$, $O$, $O_1$ (subjects) and $O_2$ (centres or items) with indicator weights (I) and the minimum-$p$ rule (M), nested and crossed designs, all their alternatives}{table.14}{supplement.pdf}}
\global\@namedef{r@S-tab:localisation}{{S15}{26}{Localisation in the nested and crossed designs with the exact tests (CvM, $\alpha =0.05$, 1000 replicates per cell, ML fits, $B=999$), with indicator weights (I) and the minimum-$p$ rule (D); the hypotheses are $H_0$, the omitted fixed term $x_1^2$, the omitted random slopes of factor 1, of factor 2 and of both factors, and the omitted factor 2. Joint decisions of the factor-specific tests: ``any'' is the share of replicates in which at least one $O_l$ rejects; ``corr.'' the share in which a correct factor rejects and no wrong factor does; ``wrong'' the share in which a wrong factor rejects and no correct factor does; ``both'' the share in which both factors reject. The correct factor is the one whose random slope is omitted from the fit: factor 1 (subjects) under ``slope 1'', factor 2 (centres or items) under ``slope 2'', both under ``slopes 1, 2'' (where every factor is correct, so ``wrong'' is 0); under $H_0$, under the omitted $x_1^2$ and under the omitted factor 2 (where only $O_1$ exists) no factor is correct and every factor-specific rejection counts as wrong. Sequential reading: $F_E$ rejects (whatever the $O$ tests do); otherwise $O$ rejects and a correct $O_l$ rejects (``$O$,c''); otherwise $O$ rejects and a wrong $O_l$ rejects (``$O$,w''); neither $F_E$ nor $O$ rejects (``none''); the remainder, $O$ rejecting without any $O_l$, is omitted. Leading zeros are omitted}{table.15}{supplement.pdf}}
\global\@namedef{r@S-tab:author-extra-weak-slopes}{{S16}{27}{An omitted subject slope at $n=4000$: minimum-$p$ CvM rejection rates of the exact tests by the generating standard deviation of the slope (the fitted model has a random intercept only at the subject level; the other random part is correctly specified). Zero standard deviation is the boundary-null control, 0.75 the slope-1 scenario of the main study; 1000 replicates per row, $B=999$, Monte Carlo standard error at most 0.016}{table.16}{supplement.pdf}}
\global\@namedef{r@S-tab:whitener-compare}{{S17}{28}{The fixed-part process with the symmetric root $\widehat {\bm V}^{-1/2}$, the whitener of $F$ (S), and with the structured factor of the one-level implementation ($F_{\rm Ch}$, C): rejection rates at $\alpha =0.05$ on the first 1000 replicates of the paper's study at $n=250$ and 1000 and the first 300 at $n=4000$ (ML fits, $B=999$, the same Gaussian draws for both), with indicator weights (I) and the minimum-$p$ rule (D); ``agree'' is the share of replicates in which the two CvM tests with the minimum-$p$ rule reach the same decision and $\overline {|\Delta p|}$ the mean absolute difference of their $p$-values. Hypotheses: $H_0$; $x_1^2$, the quadratic term omitted from the fit; slope 1, the subject slope omitted. Monte Carlo standard error of a rate at most 0.029 (0.007 at the nominal level with 1000 replicates); the paired standard error of a difference is smaller. Leading zeros are omitted}{table.17}{supplement.pdf}}
\global\@namedef{r@S-tab:whitener-timing}{{S18}{29}{Cost of the two whiteners of the fixed-part process on one replicate of every design of the study (one BLAS thread, as in the workers of the study; the minimum of two runs after a warm-up, one run at $n\ge 16\,000$): $q$ is the number of random-effect columns, ``component'' the number of columns in the largest connected component of the grouping graph, which is the dimension of the eigenproblem of the symmetric root; ``fit'' the ML fit with \texttt {MixedModels.jl}; ``build'' the construction of the package model with the symmetric root of $F$ (S) and with the structured factor of the one-level implementation (C, $F_{\rm Ch}$), and ``test'' the complete test with $B=999$, the six scales and all processes, which is the same computation after the construction. Seconds}{table.18}{supplement.pdf}}
\global\@namedef{r@S-tab:benchmark}{{S19}{30}{Rejection rates at $\alpha =0.05$ of the exact tests $F_E$, $O_E$ and the factor-specific $O_E$ tests with CvM (minimum-$p$ rule over $\lambda =c/I$, $c\in \{1,2,10,100,1000\}$), from this paper's study (the minimum-$p$ CvM entries of Tables~\ref {tab:exact-nested} and~\ref {tab:exact-crossed}), and of the tests that name the alternative, computed by the companion paper on the same 1000 replicates (ML fits, $B=999$): the Wald $z$-test of the $x_1^2$ coefficient in the fitted model augmented by $x_1^2$, and the likelihood-ratio tests $\mathrm {LRT}_l$ of one additional correlated random slope for factor $l$ (reference $\tfrac 12\chi ^2_k+\tfrac 12\chi ^2_{k+1}$, $k$ the number of random coefficients of the factor in the fitted model)}{table.19}{supplement.pdf}}
\global\@namedef{r@S-tab:factorial}{{S20}{31}{Factorial scenario with few covariate patterns: rejection rates at $\alpha =0.05$ of the $F$, $O$, $O_{\mathrm {subj}}$ and $O_{\mathrm {item}}$ tests (KS and CvM; I: indicator weights, D: minimum-$p$ rule over the scales) and the share of singular ML fits, 1000 replicates per cell, $B=999$; layouts $56\times 32$ ($n=1792$, the size of \texttt {kb07}) and $112\times 64$ ($n=7168$); fitted model $y\sim 1+a+(1+a\mid \mathrm {subj})+(1\mid \mathrm {item})$, the item slope omitted ($\tau =0$: the fitted model is correct), and the rows ``correct'' with $(1+a\mid \mathrm {item})$ at $\tau =0.5$. The data and the two degeneracies are described in the text; dashes denote processes that are identically zero in every replicate. Monte Carlo standard error at most 0.016}{table.20}{supplement.pdf}}
\global\@namedef{r@S-sec:si-exact-F}{{S6.11}{32}{The exact calibration of the fixed-part process}{subsection.6.11}{supplement.pdf}}
\global\@namedef{r@S-sec:fg-stress}{{S6.11}{32}{The exact calibration of the fixed-part process}{subsection.6.11}{supplement.pdf}}
\global\@namedef{r@S-tab:exact-F-main}{{S21}{33}{The exact test of the fixed-part process ($F_E$, Theorem~\ref {M-thm:exact-main} with the offset $\bm c_F$) against the $F$ test with unrescaled Gaussian draws, computed on the same replicates and random vectors, and against the fixed-prediction process ($O_\varnothing $: ordering $\bm X\widehat {\bm \beta }$, marks $\widehat \sigma ^{-1}\bm R\bm y$, the same rotations without the offset): CvM rejection rates at $\alpha =0.05$ with indicator weights (I) and the minimum-$p$ rule (M), 1000 replicates per cell}{table.21}{supplement.pdf}}
\global\@namedef{r@S-tab:exact-F-stress}{{S22}{33}{The omitted-slope stress designs of Section~\ref {sec:fg-stress} ($n=992$; the omitted slope has standard deviation 3 and multiplies a covariate that varies within the fitted groups, so it lies outside the fitted span): CvM rejection rates at $\alpha =0.05$ with the minimum-$p$ rule under the fixed-mean null (correct fixed mean, omitted slope) and under the mean alternative, of $F$, $F_E$ and $O_\varnothing $ as in Table~\ref {tab:exact-F-main} on the full observed-value grid with $B=999$ (1000 and 500 replicates). Leading zeros are omitted}{table.22}{supplement.pdf}}
\global\@namedef{r@S-sec:si-application}{{S7}{34}{Details of the applications}{section.7}{supplement.pdf}}
\global\@namedef{r@S-sec:si-small-studies}{{S7.1}{34}{The two small studies}{subsection.7.1}{supplement.pdf}}
\global\@namedef{r@S-sec:si-kb07}{{S7.2}{34}{A crossed response-time experiment}{subsection.7.2}{supplement.pdf}}
\global\@namedef{r@S-tab:small-studies-si}{{S23}{35}{The two small studies, all models: KS/CvM $p$-values with the minimum-$p$ rule over the five scales, $B=99\,999$ Gaussian vectors per fit. E: rotations; $G_{\rm r}$: Gaussian draws with the marks divided by the residual standard deviation; $G_{\widehat \sigma }$: Gaussian draws with the marks divided by $\widehat \sigma $ (Section~\ref {sec:si-small-r}). Joint, over $F_E$ and $O$, and $F_E$ use rotations. The gasoline models have crude intercepts and the rat models a random intercept and slope for each animal. A dagger marks a singular fit}{table.23}{supplement.pdf}}
\global\@namedef{r@S-tab:kb07-main}{{S24}{35}{Goodness-of-fit $p$-values for \texttt {kb07} (Kolmogorov--Smirnov/Cram\'er--von Mises, $B=999$, ML fits, minimum-$p$ rule over the five scales): the exact tests of Theorem~\ref {M-thm:exact-main} of the paper for the projected processes, and the joint test of Corollary~\ref {M-cor:joint-main} over the nondegenerate projected processes and the five scales, all from the same rotations. par.\ is the number of fitted parameters; the Monte Carlo standard error of a $p$-value is at most 0.016. Indicator weights and Gaussian draws are in Table~\ref {tab:kb07-gaussian}}{table.24}{supplement.pdf}}
\global\@namedef{r@S-fig:kb07-exact-main}{{S3}{36}{Projected processes for the \texttt {kb07} random-intercept model ($n=1789$, ML fit, indicator weights). Dark lines are primary processes; grey lines are 40 secondary paths from the $B=999$ rotations, shared across the three orderings. Tied thresholds are accumulated together. The overall and item orderings show departures, while the subject ordering does not. These paths illustrate the conditional law; the displayed collection is not an acceptance band. Table~\ref {tab:kb07-main} reports the tests with the minimum-$p$ rule}{figure.3}{supplement.pdf}}
\global\@namedef{r@S-tab:kb07-gaussian}{{S25}{37}{Gaussian (G) and exact (E) $p$-values of the projected processes for the \texttt {kb07} models (KS/CvM, $B=999$, ML fits, the same draws): G uses the secondary marks $\bm R\bm \xi _b$, E their rescaling $d\sqrt r\,\bm R\bm \xi _b/\|\bm R\bm \xi _b\|$ of Theorem~\ref {M-thm:exact-main} of the paper. I denotes indicator weights and D the minimum-$p$ rule; $d$ is the radial factor of the model}{table.25}{supplement.pdf}}
\global\@namedef{r@S-fig:kb07}{{S4}{38}{Processes for the \texttt {kb07} random-intercept model with indicator weights (top) and the minimum-$p$ rule over the scales (bottom; $c=2$, 2, 1 and 1 selected by the CvM rule for $F$, $O$, $O_{\rm subj}$ and $O_{\rm item}$). Black lines are the primary processes and grey bands the pointwise 2.5\% and 97.5\% quantiles of the secondary processes, so a path leaving the band is not itself a rejection; Table~\ref {tab:kb07-main} gives the tests. The $F$ panel has eight ordering values and is uninformative here (Table~\ref {tab:kb07-main}); its band is the whitened group-effect component that Gaussian draws treat as random and the exact test conditions away}{figure.4}{supplement.pdf}}
\global\@namedef{r@S-tab:kb07-reml}{{S26}{39}{Goodness-of-fit $p$-values for \texttt {kb07} with REML fits (Kolmogorov--Smirnov/Cram\'er--von Mises, $B=999$, the same secondary draws as the ML analysis): Gaussian draws for $F$ and the exact test for the projected processes. I denotes indicator weights and D the minimum-$p$ rule}{table.26}{supplement.pdf}}
\global\@namedef{r@S-fig:kb07-qq}{{S5}{39}{Normal quantile plot of the standardised projected residuals $(\bm R\bm y)_i/(\widehat \sigma R_{ii}^{1/2})$ of the \texttt {kb07} random-intercept model}{figure.5}{supplement.pdf}}
\global\@namedef{r@S-sec:si-lean}{{S8}{40}{Formal verification}{section.8}{supplement.pdf}}
\global\@namedef{r@S-tab:statement-map}{{S27}{41}{Statements of the main paper and the Lean modules that verify them; the S-numbered counterparts are listed in the guide at the start of this supplement, \texttt {lean/PROOF\_MAP.md} lists the theorem names and \texttt {lean/STATEMENT\_CHANGES.md} the recorded differences}{table.27}{supplement.pdf}}
\makeatother
